# Supplementary material for: A Comparative Study of Quality and Content-Based Spatial Pooling Strategies in Image Quality Assessment
Source: arXiv:1811.08891 ancillary file (2018-11-21)
Supplement: Supplementary file 1 [file slides.pdf]

# **A Comparative Study of Quality and Content-based Spatial Pooling Strategies in Image Quality Assessment**

Can Temel and Ghassan AlRegib\*

Multimedia and Sensors Lab (MSL)  
Center for Signal and Information Processing (CSIP)  
Georgia Institute of Technology  
December 15, 2015

1. Pixels to Perception (P2P) Issue
  - In Theory
  - In Practice
2. The Role of Pooling in P2P
  - Spatial Pooling Strategies
  - Proposed Method: Weighted Percentile Pooling (WPP)
  - Pooling in 1D
  - Pooling in 2D
3. Comparison of Spatial Pooling Strategies
4. Conclusion

# Image Quality Assessment Issue

Capture

Store

Transfer

Display

Perceive

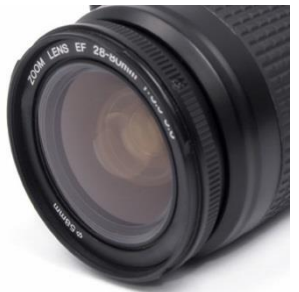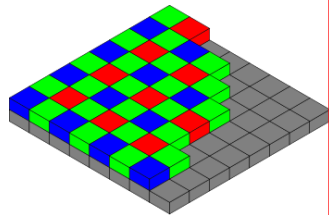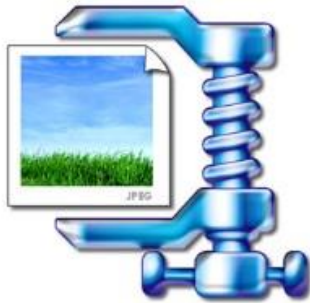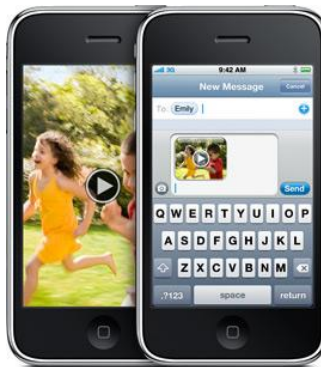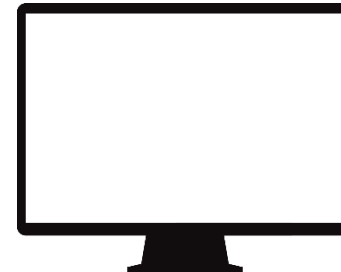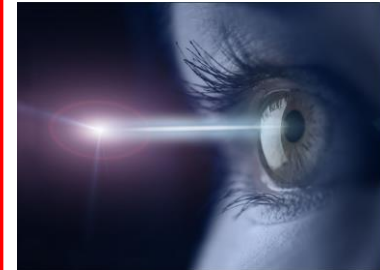

P2P

Pixels

Perception

# Databases: Off the shelf and simulated degradations

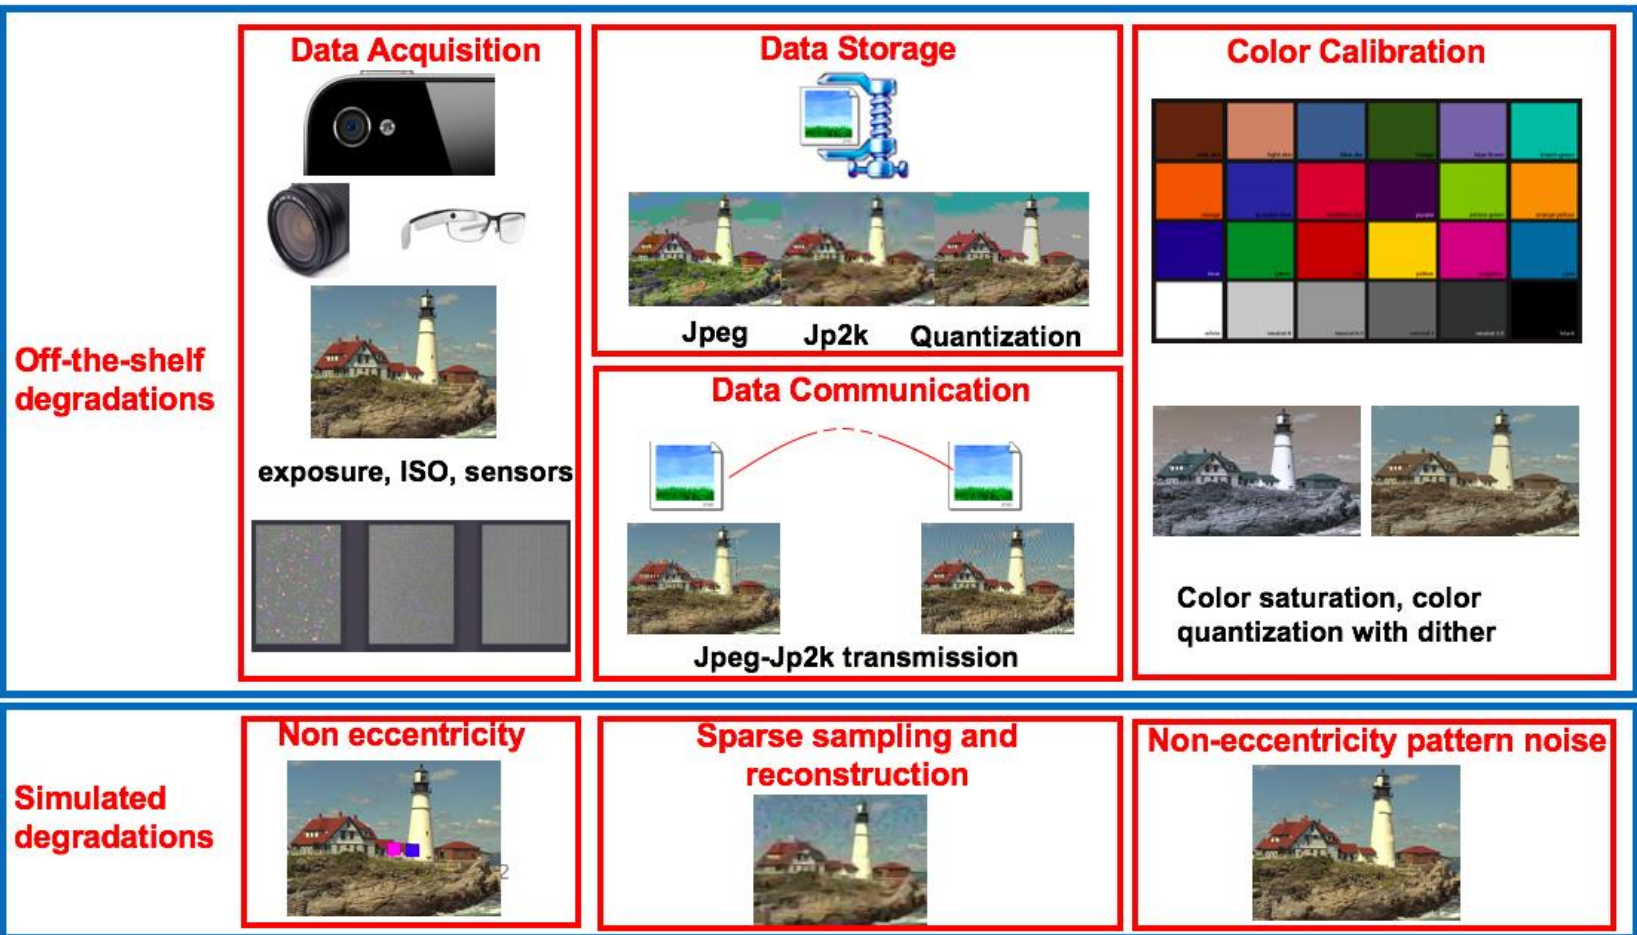

# Objective Quality Metric Types

## Full Reference (FR)

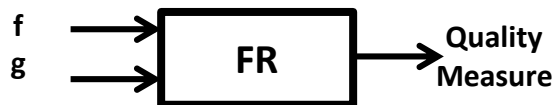

## Reduced Reference (RR)

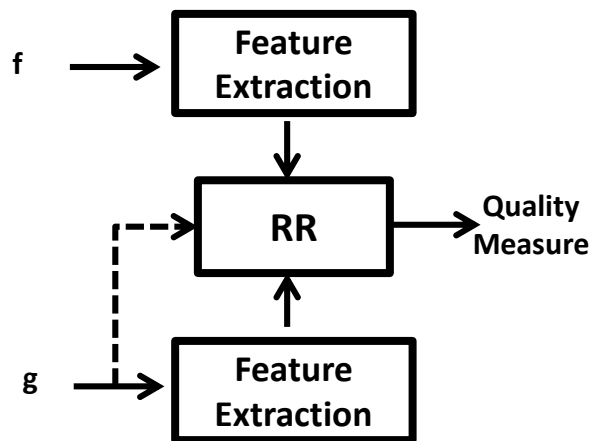

## No Reference (NR)

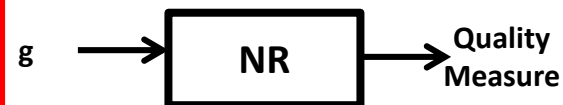

# Literature: Objective Quality Metric Types

|                                           |                                                                                                                     |
|-------------------------------------------|---------------------------------------------------------------------------------------------------------------------|
| <b>1- Basic statistics</b>                | <i>Mean, Median, Min, Max</i>                                                                                       |
| <b>2- Percentile</b> [3]                  | $\begin{cases} \frac{Q[m,n]}{z}, & Q[m,n] < \text{perc}(p, Q) \\ Q[m,n]^{c_1}, & \text{otherwise} \end{cases}$      |
| <b>3- Five Number Summary</b> [1]         | $\frac{\text{mean} + \text{perc}(25, Q) + \text{median} + \text{perc}(75, Q) + \text{max}}{5}$                      |
| <b>4- Minkowski</b> [2]                   | $\sum_{m=1}^M \sum_{n=1}^N \frac{Q[m,n]^p}{M N}$                                                                    |
| <b>5- Quality/Distortion Weighted</b> [2] | $\frac{\sum_{m=1}^M \sum_{n=1}^N w[m,n] Q[m,n]}{\sum_{m=1}^M \sum_{n=1}^N w[m,n]} \text{ where } w[m,n] = Q[m,n]^p$ |
| <b>5- Information Weighted</b> [2]        | $\log \left( \left( 1 + \frac{\sigma_I[m,n]^2}{c_2} \right) \left( 1 + \frac{\sigma_J[m,n]^2}{c_2} \right) \right)$ |

[1], C.G. Zewdie *et al.*, "A New Pooling Strategy for Image Quality Metrics: Five Number Summary," in *Visual Information Processing (EUVIP)*, 2014 5th European Workshop on , vol., no., pp.1-6, 10-12 Dec. 2014

[2] M. Gong and M. Pedersen, "Spatial Pooling for Measuring Color Printing Quality Attributes", in *Journal of Visual Communication and Image Representation*, 23(5), pp. 685-696, Jul. 2012

[3] A.K. Moorthy and A.C. Bovik, "Visual Importance Pooling for Image Quality Assessment," in *Selected Topics in Signal Processing, IEEE Journal of* , vol.3, no.2, pp.193-201, April 2009

I: Reference image, J: Compared image, Q:Quality map

# Percentile Pooling

- One threshold ( $p$ ) – needs to be tuned

$$\begin{cases} \frac{Q[m,n]}{Q[m,n]} z, & Q[m,n] < \text{perc}(p, Q) \\ Q[m,n], & \text{otherwise} \end{cases} \quad [1]$$

- One weight ( $c_1$ ) – needs to be tuned

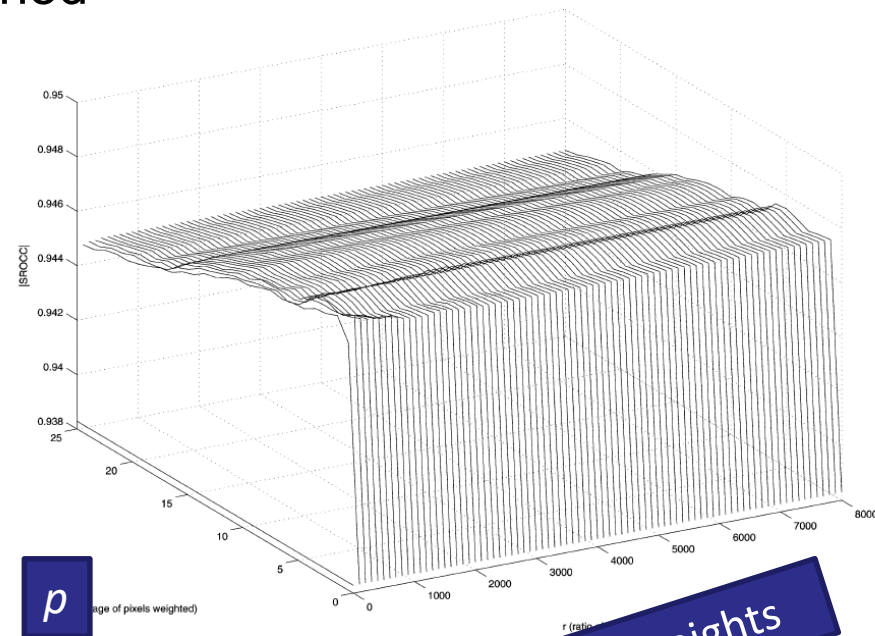

Ratio of weights

[1] A.K. Moorthy and A.C. Bovik, "Visual Importance Pooling for Image Quality Assessment," in *Selected Topics in Signal Processing*, IEEE Journal of, vol.3, no.2, pp.193-201, April 2009

$$\frac{\text{mean} + \text{perc}(25)Q + \text{median} + \text{perc}(75)Q + \text{max}}{5} \quad [1]$$
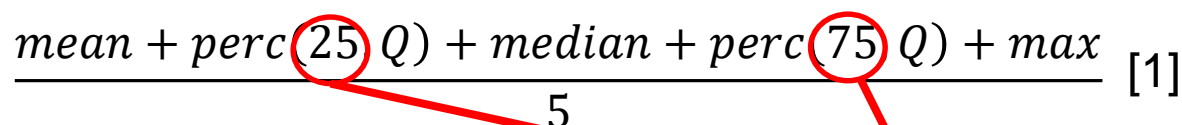

- Two constant percentile thresholds (25, 75) and their contributions are same

Based on percentile pooling and five number summary, we propose

## Weighted Percentile Pooling

- One** parameter (number of percentiles) that automatically adjusts the percentile thresholds and weights

[1] C.G. Zewdie *et al.*, "A New Pooling Strategy for Image Quality Metrics: Five Number Summary," in *Visual Information Processing (EUVIP)*, 2014 5th European Workshop on , vol., no., pp.1-6, 10-12 Dec. 2014

# Proposed pooling strategy: Weighted Percentile Pooling for Quality Maps

$$\sum_{s=1}^T \left( 1 - \frac{W_q(s)}{100} \right) \text{perc}(w_q[s], Q)$$

$$\sum_{s=1}^T \left( 1 - \frac{W_q(s)}{100} \right)$$

Only *one*  
parameter

weight-based normalization

Automatic percentile adjustment

$$w_q[s] = \begin{cases} 1 + \frac{100}{N_{bin}} s, & 1 + \frac{100}{N_{bin}} s < 100 \\ 1, & \text{otherwise} \end{cases}$$

$$s \in \mathbb{Z}$$

# Weighted Percentile Pooling: Quality Versus Distortion Maps

## Quality maps

$$\frac{\sum_{s=1}^T \left( 1 - \frac{W_q(s)}{100} \right) \text{perc}(w_q[s], Q)}{\sum_{s=1}^T \left( 1 - \frac{W_q(s)}{100} \right)}$$

$$w_q[s] = \begin{cases} 1 + \frac{100}{N_{bin}} s, & 1 + \frac{100}{N_{bin}} s < 100 \\ 1, & \text{otherwise} \end{cases}$$

## Distortion maps

$$\frac{\sum_{s=1}^T \left( \frac{W_d(s)}{100} \right) \text{perc}(w_d[s], D)}{\sum_{s=1}^T \left( \frac{W_d(s)}{100} \right)}$$

$$w_d[s] = \begin{cases} 100 - \frac{100}{N_{bin}} s, & 100 - \frac{100}{N_{bin}} s > 1 \\ 100, & \text{otherwise} \end{cases}$$

$$s \in \mathbb{Z}$$

# Pooling in 1D

$A = [4 \ 3 \ 4 \ 3 \ 4 \ 3 \ 5 \ 1 \ 2 \ 2]$

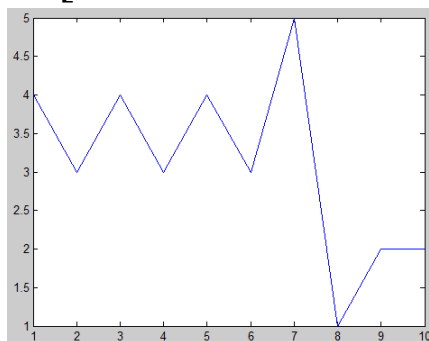

| <i>mean</i> | <i>median</i> | <i>min</i> | <i>max</i> | <i>prctile(20,2)</i> | <i>5<sub>Num</sub></i> | <i>Minkowski</i>       | <i>Qulity</i>          | <i>WPP(5)</i> |
|-------------|---------------|------------|------------|----------------------|------------------------|------------------------|------------------------|---------------|
| 3.10        | 3.00          | 1.00       | 5.00       | 2.95                 | 3.42                   | $1/8 \rightarrow 1.14$ | <i>/Distortion</i>     | 2.13          |
|             |               |            |            |                      |                        | $1/4 \rightarrow 1.30$ | $1/8 \rightarrow 3.16$ |               |
|             |               |            |            |                      |                        | $1/2 \rightarrow 1.72$ | $1/4 \rightarrow 3.21$ |               |
|             |               |            |            |                      |                        | $2 \rightarrow 10.90$  | $1/2 \rightarrow 3.32$ |               |
|             |               |            |            |                      |                        | $4 \rightarrow 166.90$ | $1 \rightarrow 3.51$   |               |
|             |               |            |            |                      |                        | $8 \rightarrow 60,743$ | $2 \rightarrow 3.80$   |               |
|             |               |            |            |                      |                        |                        | $4 \rightarrow 4.18$   |               |
|             |               |            |            |                      |                        |                        | $8 \rightarrow 4.60$   |               |

# Pooling in 2D

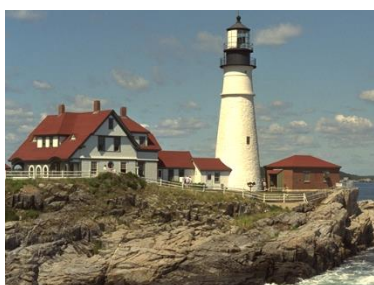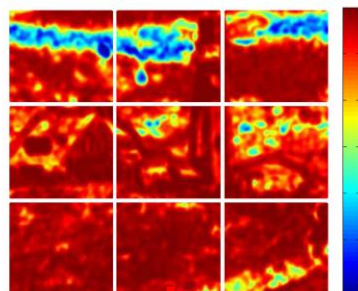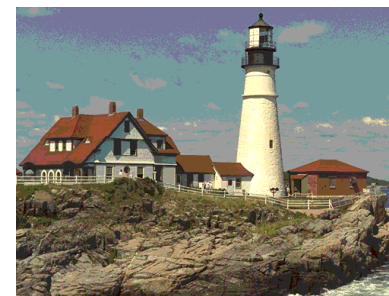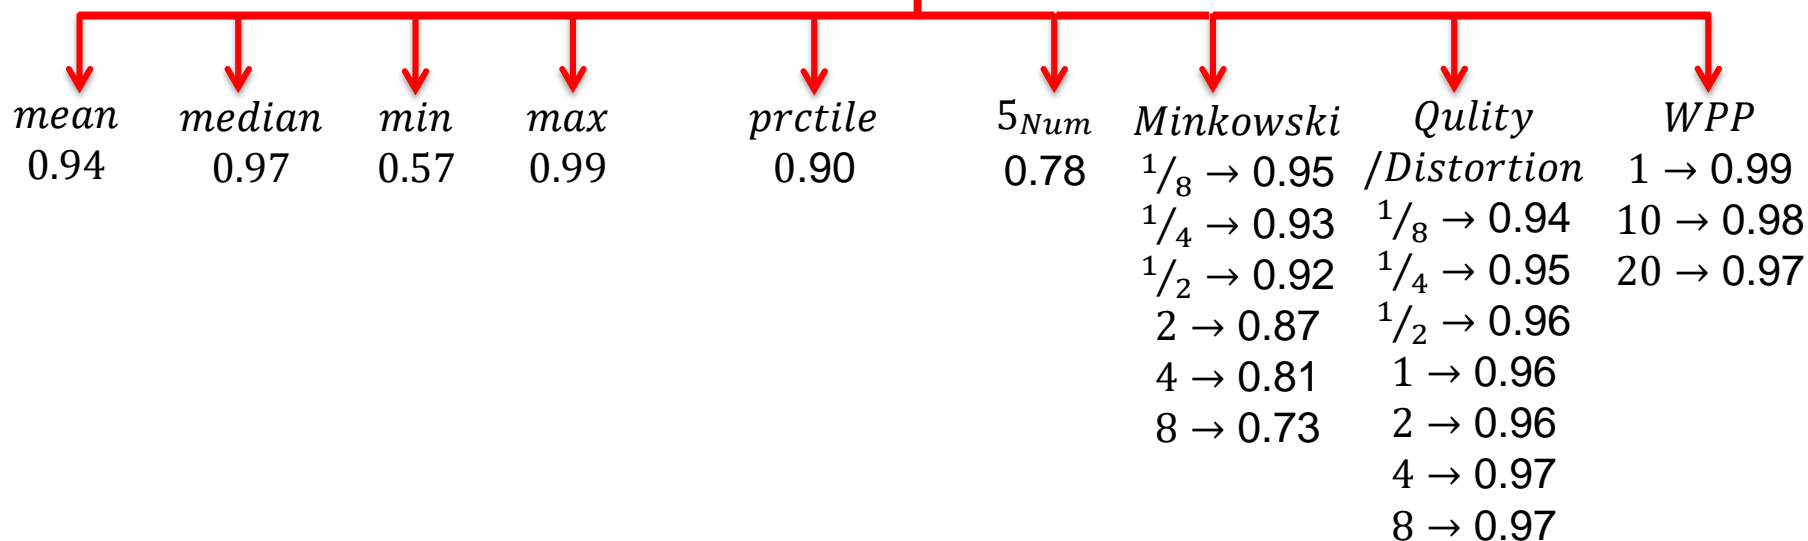

| Artifact type \<br>Databases | LIVE | MULTI | TID2013 | TOTAL |
|------------------------------|------|-------|---------|-------|
| Compression                  | 460  | 225   | 375     | 1060  |
| Noise                        | 174  | 225   | 1375    | 1774  |
| Communication                | 174  | -     | 250     | 424   |
| Blur                         | 174  | 450   | 250     | 874   |
| Color                        | -    | -     | 375     | 375   |
| Global                       | -    | -     | 250     | 250   |
| Local                        | -    | -     | 250     | 250   |

# Quality Metrics: Squared Error, SSIM and PerSIM

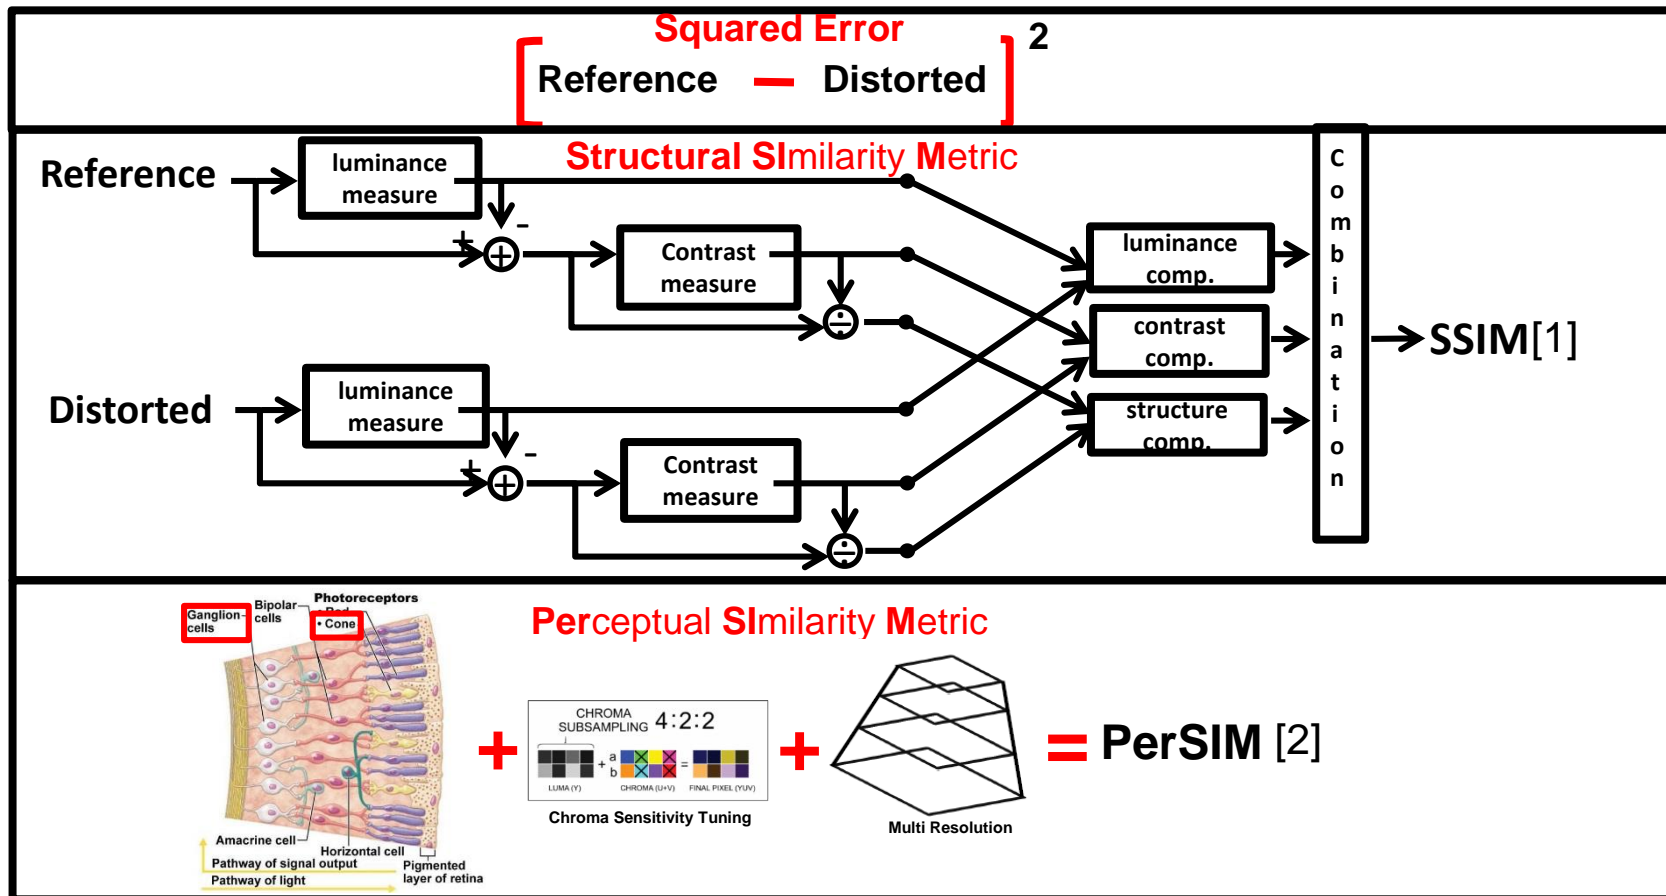

[1] Z. Wang *et al.*, "Image Quality Assessment: From Error Visibility to Structural Similarity," in *Image Processing, IEEE Transactions on*, vol.13, no.4, pp.600-612, April 2004

[2] D. Temel and G. AlRegib, "PerSIM: Multi-Resolution Image Quality Assessment in the Perceptually Uniform Color Domain," *Image Processing (ICIP), 2015 22th IEEE International Conference on*, 2015.

# Validation metrics: Pearson and correlation coefficient

Pearson

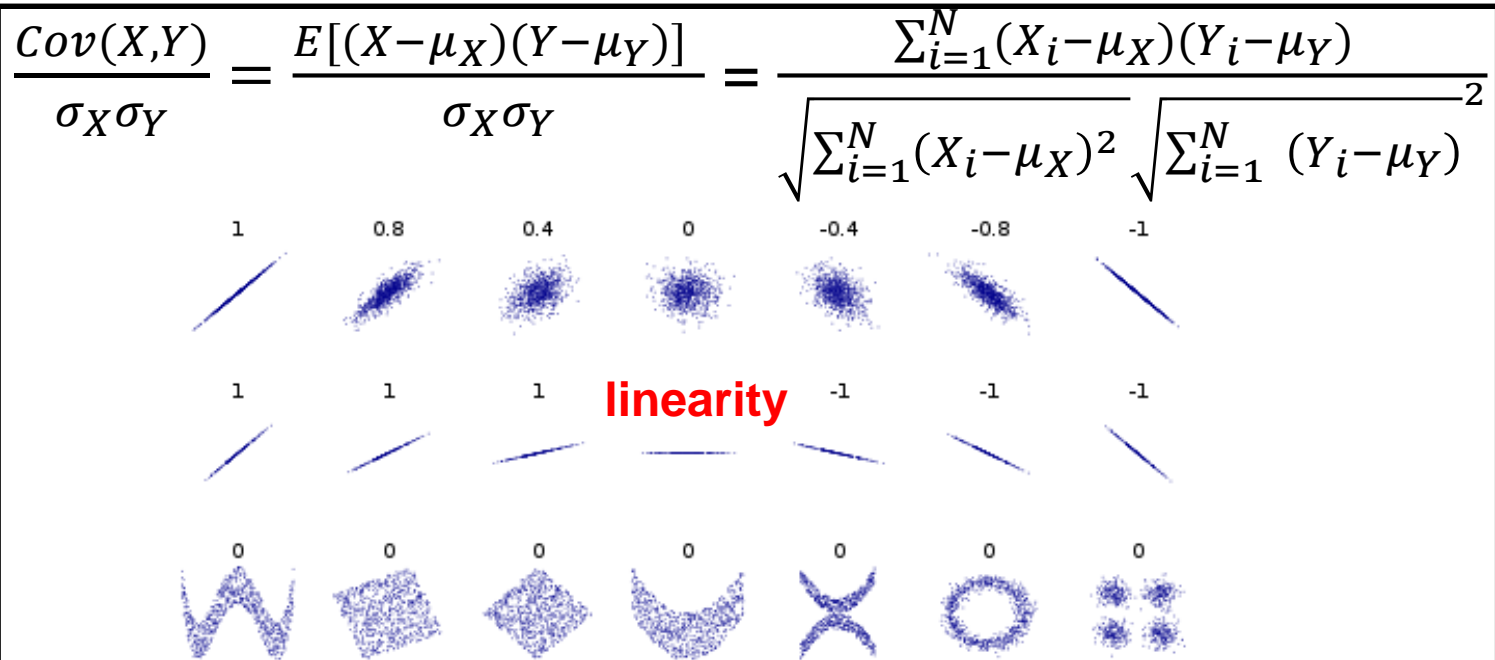

Spearman

$$X_i, Y_i \longrightarrow x_i, y_i$$

monotonicity

$$1 - \frac{6 \sum_{i=1}^N (x_i - y_i)^2}{N(N^2 - 1)}$$

# Results: LIVE database

- **Pearson:** Percentile and weighted percentile pooling are the best in the full database
- **Spearman:** Information weighted and weighted percentile pooling using SSIM are the best

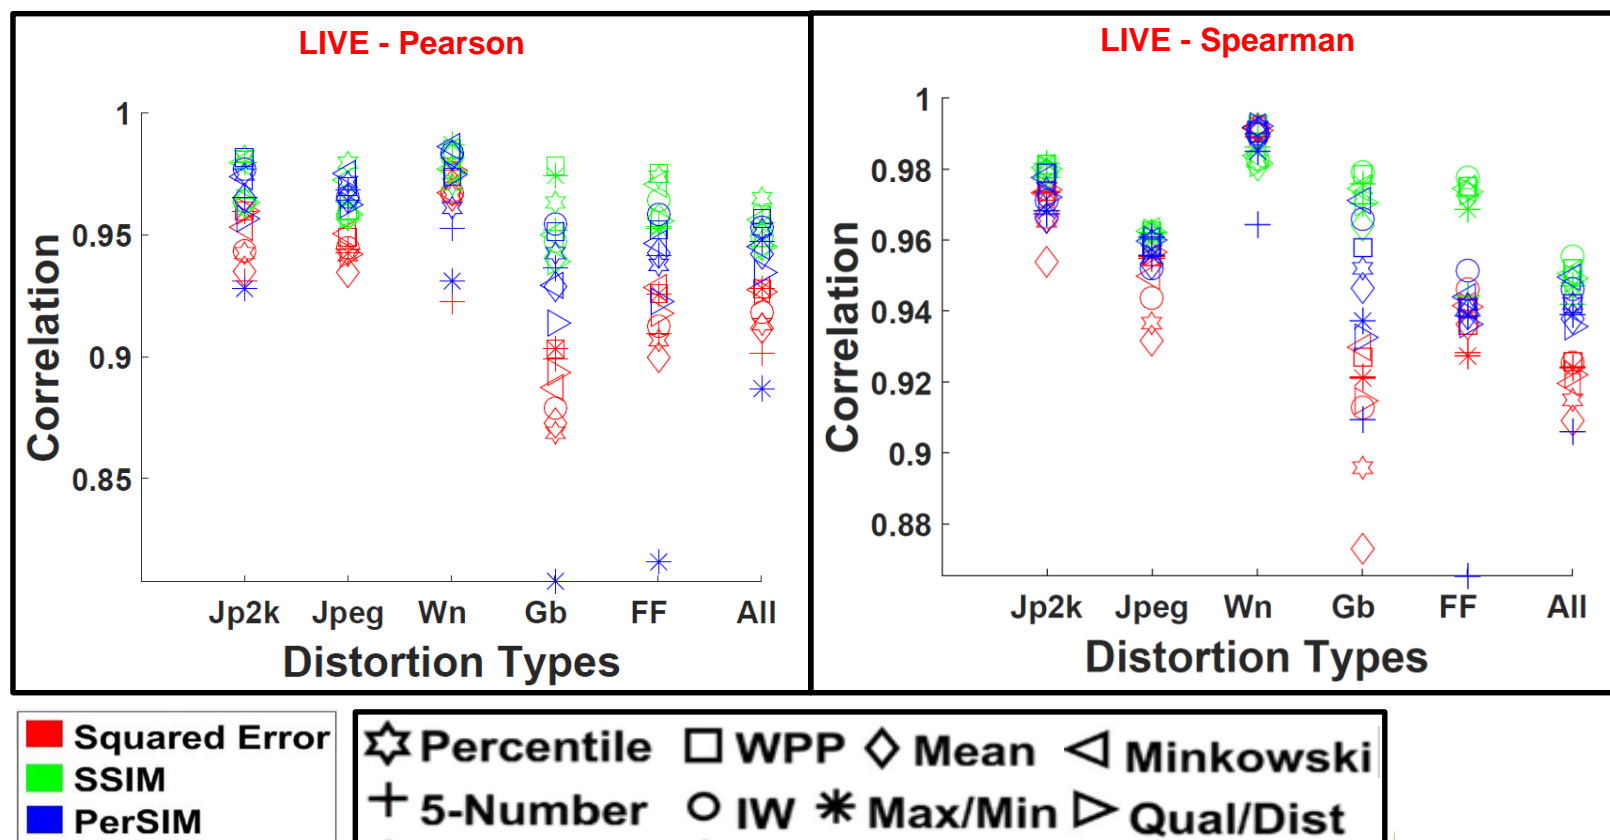

# Results: MULTI database

- **Pearson:** Minkowski and Max/min are the best for SSIM, information-weighted and weighted percentile pooling are the best for PerSIM, percentile is the best for squared error
- **Spearman:** Information weighted and max/min are the best for SSIM, weighted percentile pooling is the best for PerSIM

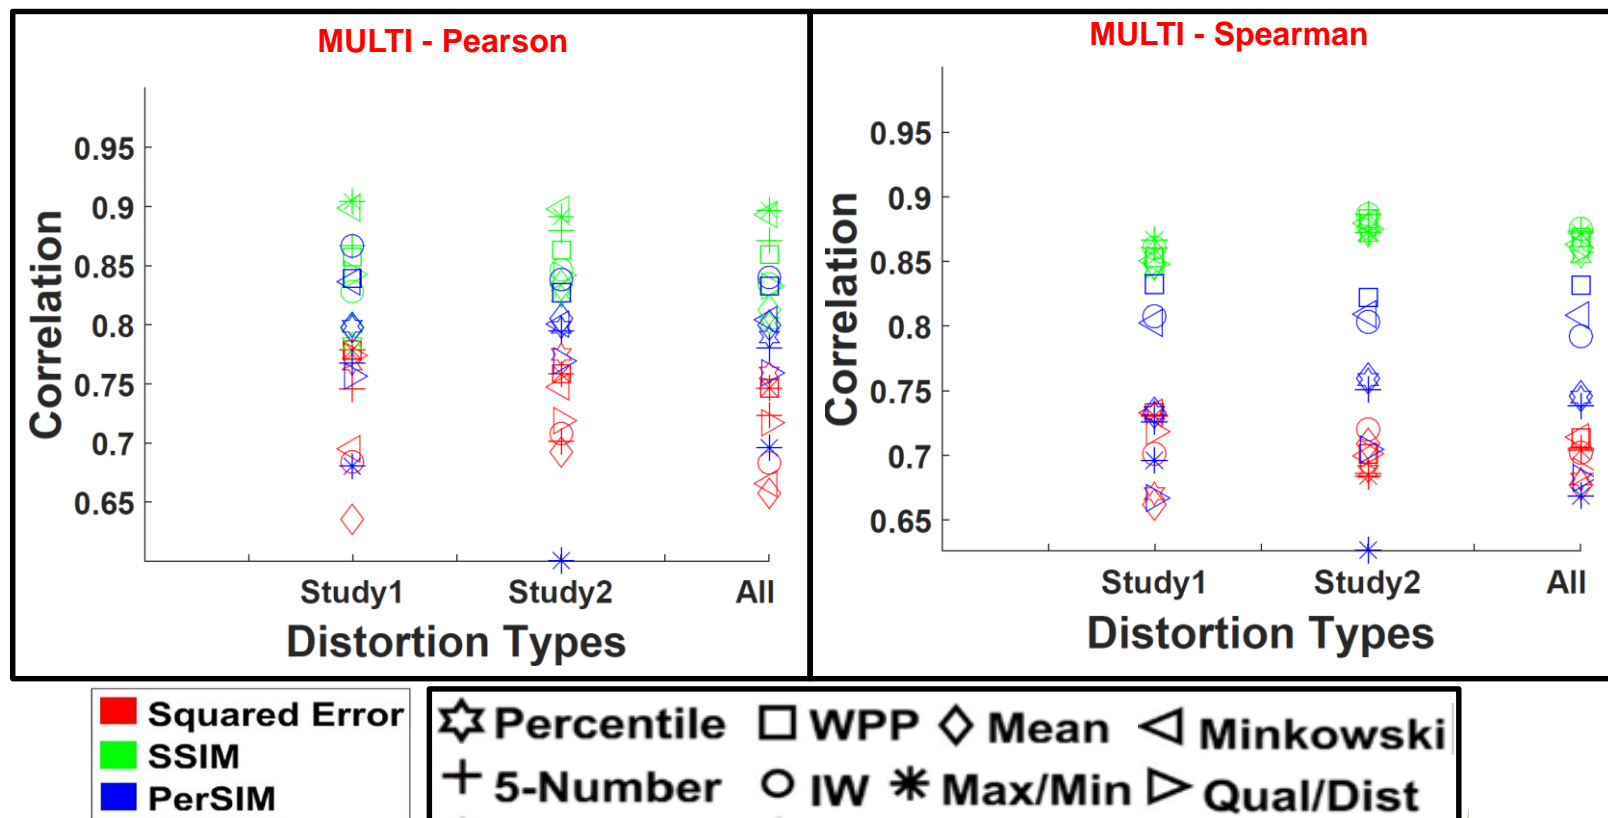

# Results: TID13 database

- **Pearson:** Weighted percentile pooling is the best for PerSIM
- **Spearman:** Minkowski pooling is the best for PerSIM followed by weighted percentile pooling

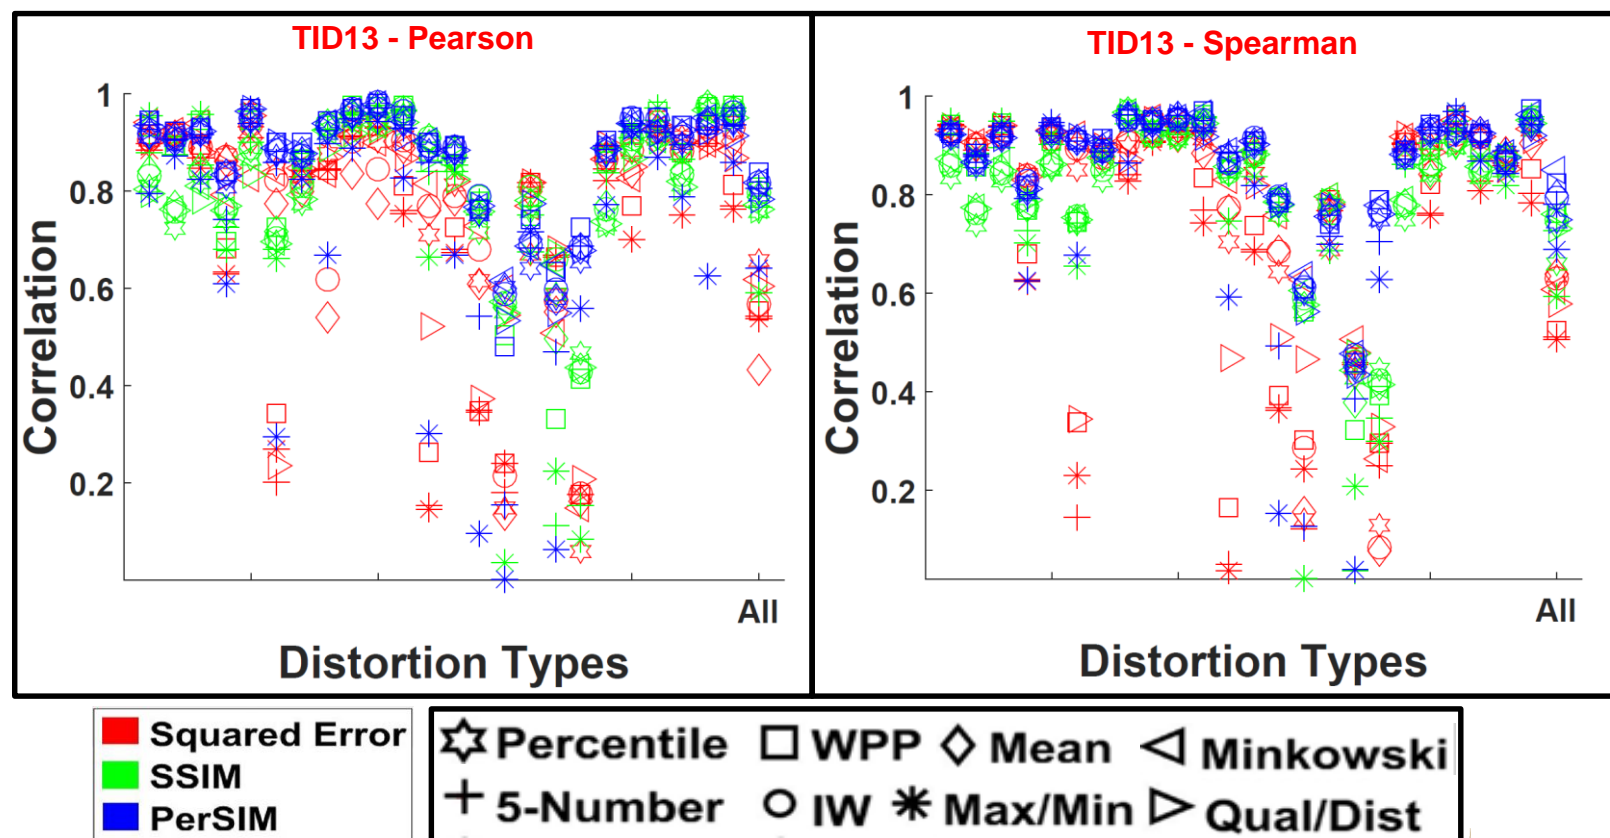

# Results: Statistical Significance

- The effect of pooling strategy selection is more significant when there are more distortion types in the validation database.

| Artifact type \ Databases | LIVE | MULTI | TID2013 |
|---------------------------|------|-------|---------|
| Compression               | 460  | 225   | 375     |
| Noise                     | 174  | 225   | 1375    |
| Communication             | 174  | -     | 250     |
| Blur                      | 174  | 450   | 250     |
| Color                     | -    | -     | 375     |
| Global                    | -    | -     | 250     |
| Local                     | -    | -     | 250     |

3 types of artifacts

**M-LIVE**

66

4 types of artifacts

**LIVE**

90

7 types of artifacts

**TID13**

116

# Results: Statistical Significance

- Structural and perceptual similarity metrics are better for differentiating pooling strategies compared to pixel-wise squared error

|          | SE | SSIM | PerSIM |
|----------|----|------|--------|
| M-LIVE   | 26 | 32   | 32     |
| LIVE     | 8  | 30   | 28     |
| TID 2013 | 34 | 38   | 44     |

- Weighted percentile pooling enhances percentile-based methods by automatically adjusting thresholds and weights.
- Pooling matters, but not as much as quality attribute design.
- Structural and perceptual similarity metrics are better for differentiating pooling strategies compared to pixel-wise squared error.
- Pooling strategy and quality attributes can not be considered as independent processes.
- The effect of pooling strategy is more significant when the distortion types are diverse.
